# Supplementary material for: Theoretical Characterization of Structural Disorder in the Tetramer Model Structure of Eumelanin
Source: arXiv:1902.09398 source file (2019-02-25)
Supplement: Supplementary file 1 [file supplementary.pdf]

# Supporting Information for: Theoretical Characterization of Structural Disorder in the Tetramer Model Structure of Eumelanin

Oleg Sapunkov, Abhishek Khetan, Vikram Pande, and Venkatasubramanian Viswanathan
*Department of Mechanical Engineering, Carnegie Mellon University.*

(Dated: February 23, 2019)

## I. FORMATION ENTHALPIES OF MONOMERS AND TETRAMERS

The primary molecular structure considered for this study was the double eumelanin tetramer. Double tetramers included in this study's simulations were built up from 3 types of eumelanin monomers: hydroquinone (HQ), indolequinone (IQ), and quinone-methide (MQ). To accurately compute interaction coefficients among the monomers within the tetramers, it was necessary to separately calculate the DFT formation energies of both the monomers and the double tetramers' constituent single tetramers. These formation energies were computed using the atomic reference, and are reported below. Further in the study, these formation enthalpies were used to compute occupation and in-plane interaction coefficients of the Ising Model.

| Monomer | $\mu$ ΔH | $\sigma$ ΔH |
|---|---|---|
| H | -2.72 | 0.19 |
| I | -1.03 | 0.26 |
| M | -0.63 | 0.30 |

TABLE S1. Atomistic formation enthalpies of the 3 monomers used in this study. It is important to note that these formation enthalpies were computed for stable, standalone monomers, with a complete set of carbon-bound hydrogens, since these form the basis of polymer formation in solution. During polymerization, two of these hydrogens are lost, and that loss was accounted for in the calculation of occupation energy terms of single and double tetramers.

## II. FORMATION ENTHALPIES OF DOUBLE TETRAMERS

Formation enthalpies of a selection of double eumelanin tetramers are presented below. These are separated into two subsections: double tetramers with a majority of hydroquinone monomers (at least 5 of 8 monomers), and double tetramers with a minority of hydroquinone monomers (at most 3 of 8 monomers). The strong dependence of formation enthalpy on HQ monomer abundance can be easily observed in the presented data, with a difference of over 12 eV between the all-HQ double tetramer and the presented HQ-free double tetramers. This dependence is best reflected in the occupation and in-plane interaction terms of the Ising Model developed for the double eumelanin tetramer presented in the main work.

| Tetramer | $\mu$ ΔH | $\sigma$ ΔH |
|---|---|---|
| HHHH | -8.66 | 0.90 |
| HHHI | -7.21 | 0.95 |
| HHHM | -7.97 | 0.94 |
| HHII | -5.65 | 1.00 |
| HHIM | -6.38 | 1.00 |
| HHMM | -6.41 | 1.01 |
| HIHI | -5.67 | 1.01 |
| HIHM | -6.51 | 1.00 |
| HMHM | -6.88 | 1.00 |
| IHIM | -4.90 | 1.04 |
| IIHM | -5.02 | 1.05 |
| IIIH | -4.00 | 1.08 |
| IIII | -2.31 | 1.15 |
| IIIM | -3.33 | 1.13 |
| IIMM | -3.41 | 1.14 |
| IMIM | -3.84 | 1.15 |
| MMIH | -4.98 | 1.06 |
| MMMH | -4.31 | 1.13 |
| MMMI | -2.83 | 1.21 |
| MMMM | -1.53 | 1.30 |

TABLE S2. Atomistic formation enthalpies of the 20 single tetramers used in this study. As can be observed, single tetramers with the highest fraction of HQ monomers have the lowest formation enthalpies, and observation that remains consistent for formation enthalpies of double tetramers as well.

| Doub.Tetrm. | $\mu$ ΔH | $\sigma$ ΔH |
|---|---|---|
| HHHH-HHHH | -19.35 | 2.81 |
| HHHH-HHHI | -18.38 | 2.81 |
| HIHH-HHHH | -18.35 | 2.83 |
| HHHH-HHHM | -18.31 | 2.78 |
| HHHH-HHIH | -18.24 | 2.82 |
| MHHH-HHHH | -17.99 | 2.79 |
| HHHH-HMHM | -17.39 | 2.89 |
| HHHH-HIHM | -17.27 | 2.83 |
| HHHH-HHMI | -17.26 | 2.81 |
| HIHH-HHHI | -17.25 | 2.86 |
| HHHI-HHIH | -17.25 | 2.87 |
| HHHH-HMHI | -17.24 | 2.83 |
| HHHH-HIHI | -17.21 | 2.86 |
| HHHH-HHII | -17.12 | 2.87 |
| HHHH-HHIM | -17.07 | 2.84 |
| MMHH-HHHH | -16.86 | 2.86 |
| HHHH-HHMM | -16.78 | 2.90 |
| HHHI-HHHI | -16.57 | 2.79 |
| HHHM-HMHI | -16.07 | 2.86 |
| HHHM-HMHM | -16.05 | 2.85 |
| HHHH-HMII | -16.04 | 2.86 |
| HHHH-HIIM | -15.96 | 2.88 |
| HHHI-HIHM | -15.81 | 2.83 |
| HHHH-HMMI | -15.79 | 2.90 |
| IHMM-HHHH | -15.79 | 2.91 |
| HHHI-HHIM | -15.62 | 2.84 |
| HHHM-HHMM | -15.59 | 2.84 |
| HHHI-HIHI | -15.40 | 2.84 |
| HHHI-HHII | -15.36 | 2.85 |

TABLE S3. Atomistic formation enthalpies of representative HQ-rich tetramers used in this study. As can be observed, double tetramers with the highest fraction of HQ monomers have the greatest formation enthalpies.

## III. PREDICTED FORMATION ENTHALPY HISTOGRAMS

Histogram plots of formation enthalpies of the full double tetramer phase space highlight the difference in the predictions provided by the 1-Step Ising Model and the 3-Step Ising Model developed to describe the double eumelanin tetramer. Both methods predict formation enthalpies within the same population bound, and with a similar population mean. However, the 1-Step model over-predicts the dependence of formation enthalpy on hydroquinone abundance, and thus coalesces the histogram primarily around several strong peaks, corresponding to HQ abundance from 0 to 8 monomers within the investigated tetramers. The 3-Step model diminishes this overprediction by smoothing out the distribution, especially in the high-HQ abundance region, making the full histogram closer to a regular Gaussian distribution. Intermediate structures with partial HQ filling are better described by this 3-Step model, as are the single tetramers, which the 1-Step model fails to predict accurate formation enthalpies for.

| Doub.Tetrm. | $\mu$ ΔH | $\sigma$ ΔH |
|---|---|---|
| IMMH-HMHM | -13.21 | 2.96 |
| IHII-MMHH | -12.88 | 3.00 |
| MHHI-HMMI | -12.83 | 2.97 |
| MMMM-HHHH | -12.46 | 2.99 |
| HIIH-MHMM | -12.41 | 3.00 |
| HHII-MMMH | -12.28 | 3.05 |
| HMHM-HMMM | -12.22 | 3.00 |
| HHHI-MMMI | -12.14 | 3.01 |
| MMMH-MMHH | -11.76 | 3.00 |
| HHMM-HMMM | -11.76 | 3.01 |
| IHIM-IHIM | -11.49 | 2.82 |
| MMHI-MMHI | -11.47 | 2.84 |
| MMII-MMHH | -11.38 | 3.02 |
| MMMH-IHMI | -11.10 | 3.02 |
| MMMM-MHHH | -11.04 | 3.08 |
| MMMH-MMMH | -9.47 | 3.13 |
| MMII-MMMH | -9.12 | 3.08 |
| MMMM-MMHH | -9.06 | 3.14 |
| MMMI-MMMH | -8.42 | 3.12 |
| MMMH-IMMM | -8.05 | 3.07 |
| MMMM-MMMH | -6.80 | 3.23 |
| MMII-IIII | -6.11 | 2.92 |
| MMMM-MMMI | -5.22 | 3.26 |

TABLE S4. Atomistic formation enthalpies of representative HQ-poor tetramers used in this study. As can be observed, double tetramers with the lowest fraction of HQ monomers have the smallest formation enthalpies.

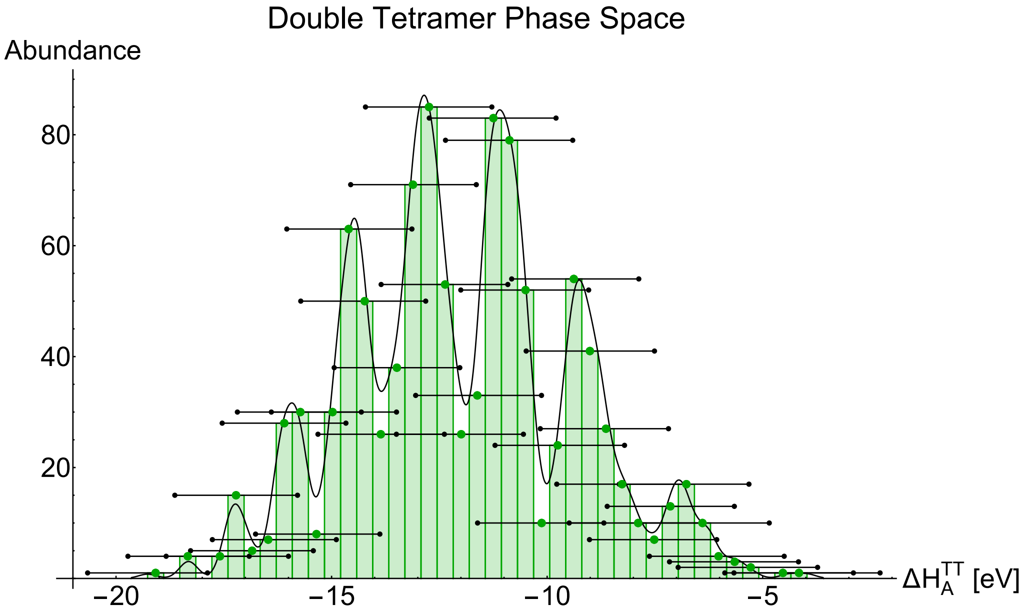


FIG. S1. Predicted formation enthalpies of the full double tetramer phase space using the 1-step computational method. Strong reliance on tetramer configuration can be seen, with well-defined peaks corresponding to individual families of tetramers, identified by the presence of discrete numbers of hydroquinone monomers in their structure.

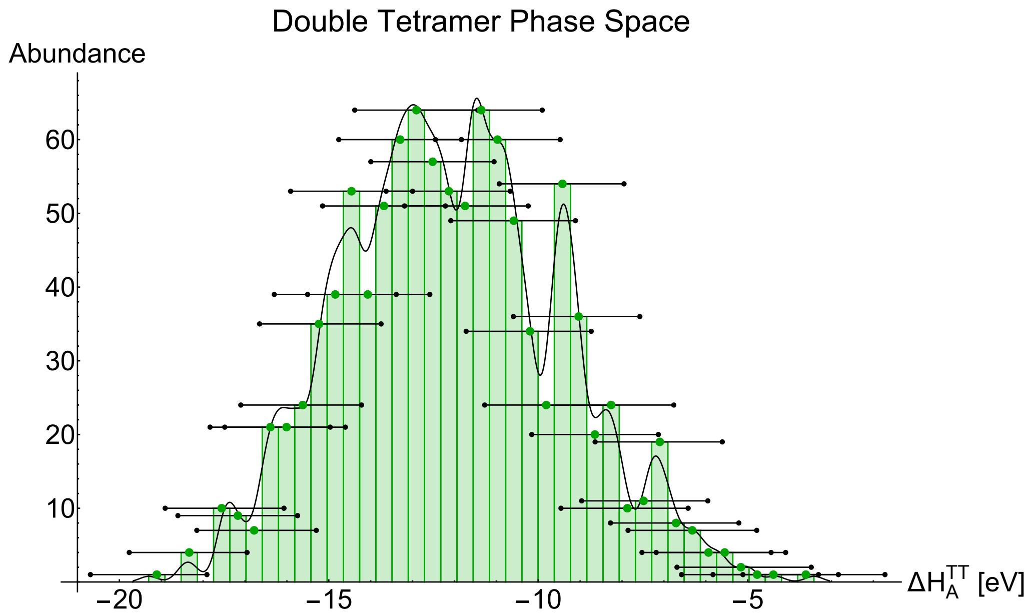


FIG. S2. Predicted formation enthalpies of the full double tetramer phase space using the 3-step computational method. Weak reliance on tetramer configuration can be seen, with a comparatively continuous distribution of formation enthalpies across the families of tetramers.
